# Supplementary material for: Human-Aligned Procedural Level Generation Reinforcement Learning via Text-Level-Sketch Shared Representation
Source: arXiv:2508.09860 source file (2026-07-17)
Supplement: Supplementary file 1 [file dataset.tex]

\begin{table*}[H]
\small
\centering
\caption{Examples from the human dataset $\mathcal{D}_\mathrm{human}$, illustrating various textual instructions and visualized levels for each task. Task conditions are highlighted in the text.}
\label{tab:dataset_human}
\vspace{0.3cm}
\begin{tabular}{@{} p{3.3cm} p{8.5cm} p{4.2cm}@{}}
\toprule
\textbf{Task} & \textbf{Text}  & \textbf{Level} \\

\midrule 
\multirow{3}{*}{\raisebox{-4em}{\textbf{Number of Regions}}}
& \multirow{2}{*}{\shortstack[l]{
    A \textit{\textbf{small\hidden{(5)}}}  cluster of \textbf{\textit{small\hidden{(5)}}} regions.\\
    A \textit{\textbf{few\hidden{(5)}}} \textbf{\textit{small\hidden{(5)}}} regions are present.%
  }
}
& \tripleimage{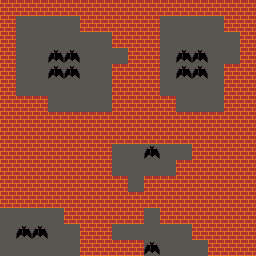}{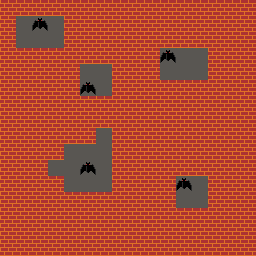}{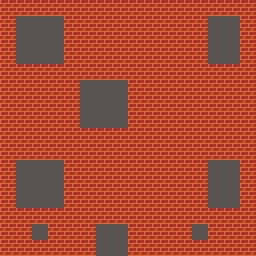} \vspace{0.03cm}\\

& \multirow{2}{*}{\shortstack[l]{
    The map has \textit{\textbf{some\hidden{(15)}}} \textit{\textbf{large}} regions.\\
   A \textit{\textbf{moderate\hidden{(15)}}} amount of \textit{\textbf{large}} regions exist.%
  }
}
& \tripleimage{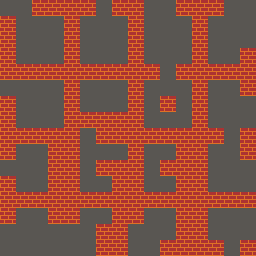}{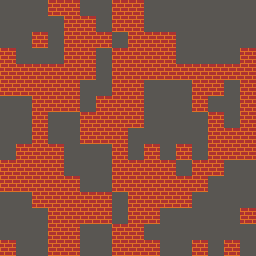}{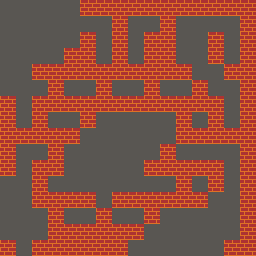} \vspace{0.03cm}\\

& \multirow{2}{*}{\shortstack[l]{
    The map contains \textit{\textbf{multiple\hidden{(25)}}} placed \textit{\textbf{small}} regions.\\
   \textit{\textbf{Small}} regions show \textit{\textbf{balanced distribution\hidden{(25)}}}.%
  }
}
& \tripleimage{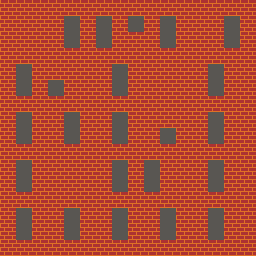}{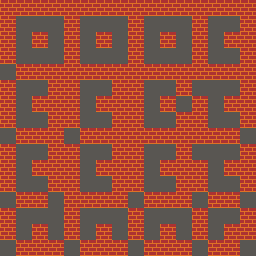}{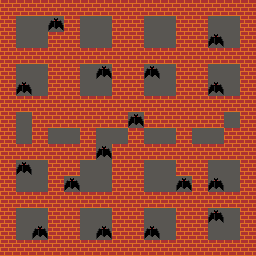} \\

\midrule 
\multirow{3}{*}{\raisebox{-4em}{\textbf{Path Length}}}
& \multirow{2}{*}{\shortstack[l]{
    \textit{\textbf{Micro\hidden{(10)}}} path length using a \textit{\textbf{narrow}} corridor.\\
    \textit{\textbf{Minimal\hidden{(10)}}} \textit{\textbf{narrow}} path requiring almost no movement.%
  }
}
&\tripleimage{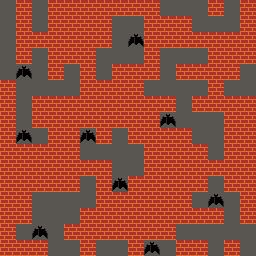}{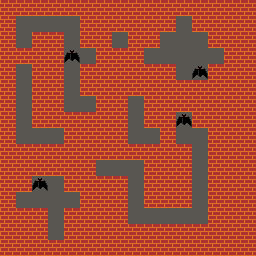}{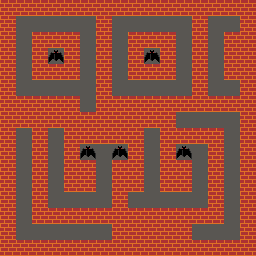} \vspace{0.03cm}\\

& \multirow{2}{*}{\shortstack[l]{
    \textit{\textbf{Brief and compact\hidden{(20)}}} \textit{\textbf{wide}} path layout.\\
    \textit{\textbf{Short\hidden{(20)}}} path length with a \textit{\textbf{wide}} design.%
  }
}
&\tripleimage{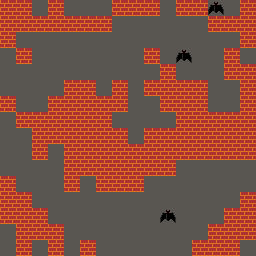}{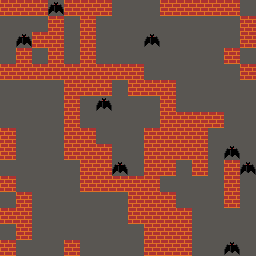}{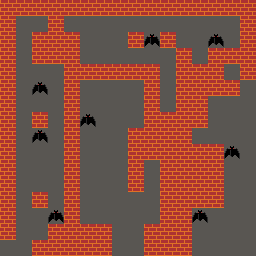} \vspace{0.03cm}\\

& \multirow{2}{*}{\shortstack[l]{
    \textit{\textbf{Moderate\hidden{(40)}}} path length along a \textit{\textbf{narrow}} path.\\
   A \textit{\textbf{medium\hidden{(40)}}}-length \textit{\textbf{narrow}} path appears on the map.%
  }
}
&\tripleimage{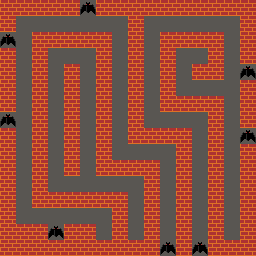}{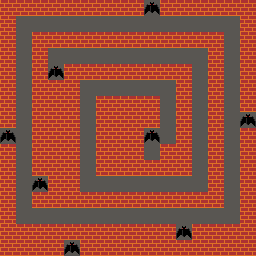}{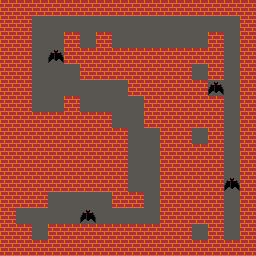} \\

\midrule 
\multirow{3}{*}{\raisebox{-4em}{\textbf{Wall Distribution}}}
& \multirow{2}{*}{\shortstack[l]{
    \textit{\textbf{Minimal\hidden{(40)}}} \textit{\textbf{decentralized}} block placement is observed.\\
    \textit{\textbf{Sparse\hidden{(40)}}} and \textit{\textbf{decentralized}} blocks occupy the map.%
  }
}
&\tripleimage{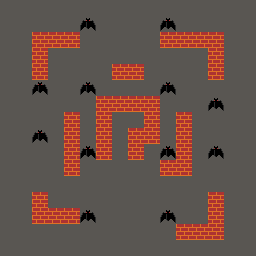}{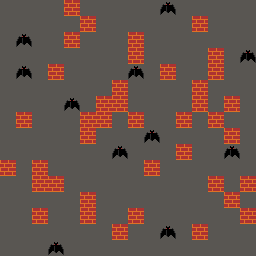}{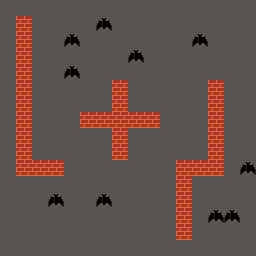} \vspace{0.03cm}\\

& \multirow{2}{*}{\shortstack[l]{
    \textit{\textbf{Some\hidden{(80)}}} \textit{\textbf{centralized}} blocks form a balanced pattern.\\
   \textit{\textbf{Centralized}} blocks appear with \textit{\textbf{moderate\hidden{(80)}}} density.%
  }
}
&\tripleimage{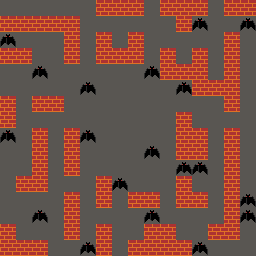}{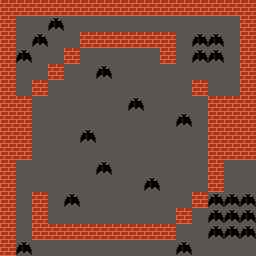}{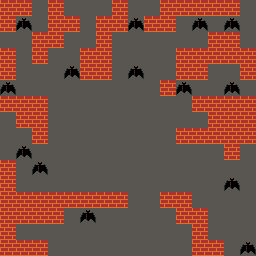} \vspace{0.03cm}\\

& \multirow{2}{*}{\shortstack[l]{
    The \textit{\textbf{decentralized}} blocks create \textit{\textbf{dense\hidden{(120)}}} barriers.\\
   \textit{\textbf{Dense\hidden{(120)}}} \textit{\textbf{decentralized}} blocks fill the area.%
  }
}
&\tripleimage{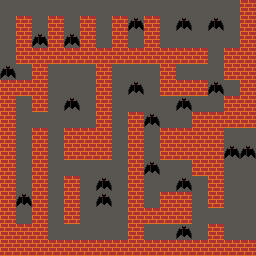}{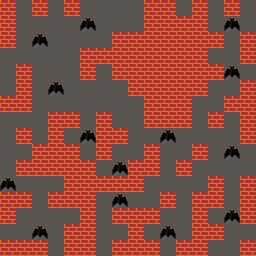}{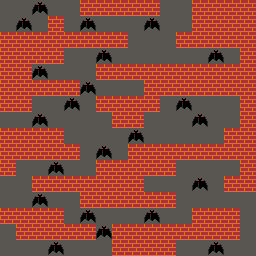}\\

\midrule 
\multirow{3}{*}{\raisebox{-4em}{\textbf{Monster Distribution}}}
& \multirow{2}{*}{\shortstack[l]{
    A \textit{\textbf{few\hidden{(10)}}} \textit{\textbf{scattered}} bats appear.\\
    \textit{\textbf{Small\hidden{(10)}}} \textit{\textbf{scattered}} bat group spotted.%
  }
}
&\tripleimage{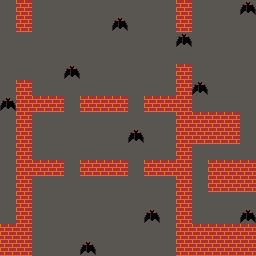}{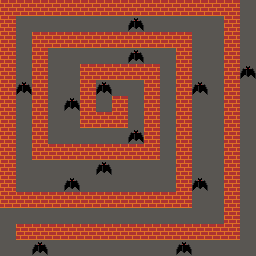}{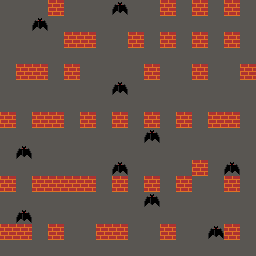} \vspace{0.03cm}\\

& \multirow{2}{*}{\shortstack[l]{
    \textit{\textbf{Some\hidden{(40)}}} \textit{\textbf{clustered}} bats spawn throughout.\\
   The map contains \textit{\textbf{several\hidden{(40)}}} \textit{\textbf{clustered}} bats.%
  }
}
&\tripleimage{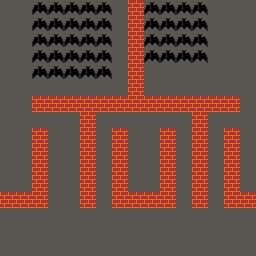}{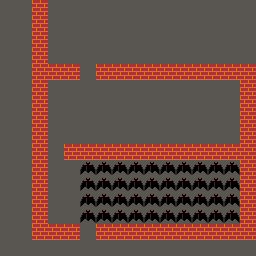}{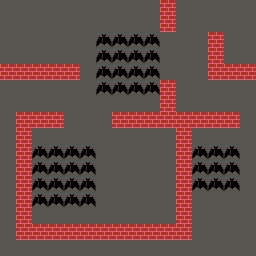} \vspace{0.03cm}\\

& \multirow{2}{*}{\shortstack[l]{
    A \textit{\textbf{dense\hidden{(70)}}} group of \textit{\textbf{scattered}} bats appears.\\
   A \textit{\textbf{multi\hidden{(70)}}}-bat \textit{\textbf{scattered}} group is seen.%
  }
}
&\tripleimage{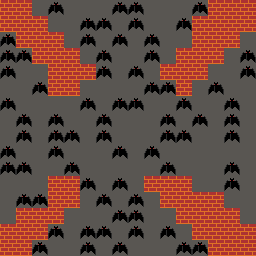}{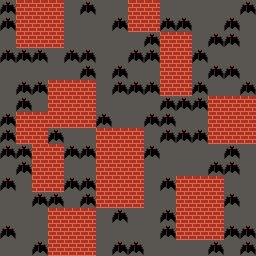}{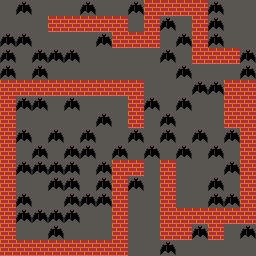}  \\

\midrule 
\multirow{3}{*}{\raisebox{-4em}{\textbf{Monster Direction}}}

& \multirow{2}{*}{\shortstack[l]{
   \textit{\textbf{Radial}} bats occupy the \textit{\textbf{western}} zone.\\
   A \textit{\textbf{radial}} formation of bats appears on the \textit{\textbf{left}}. %
  }
}
&\tripleimage{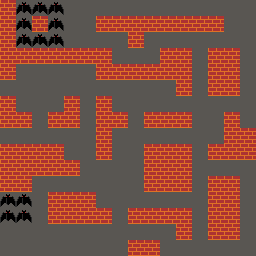}{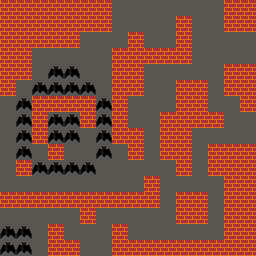}{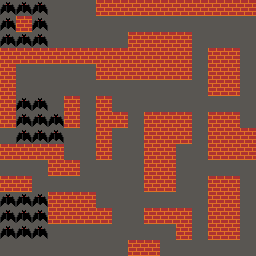} \vspace{0.03cm}\\

& \multirow{2}{*}{\shortstack[l]{
   Bats are grouped in the \textit{\textbf{north}} in a \textit{\textbf{linear}} layout.\\
   \textit{\textbf{Linear}} bats dominate the \textit{\textbf{upper}} section.%
  }
}
&\tripleimage{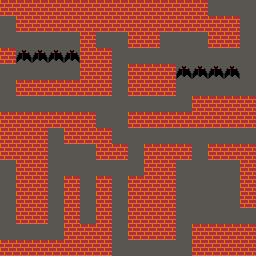}{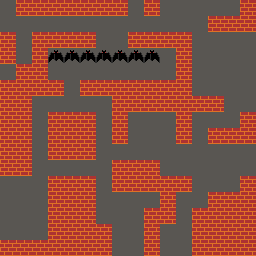}{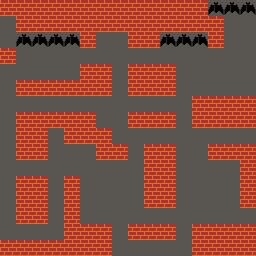} \vspace{0.03cm}\\

& \multirow{2}{*}{\shortstack[l]{
    \textit{\textbf{Radial}} bats formation appears on the \textit{\textbf{right}}.\\
   Bats in the \textit{\textbf{east}} follow a \textit{\textbf{radial}} distribution.%
  }
}
&\tripleimage{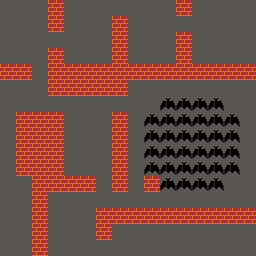}{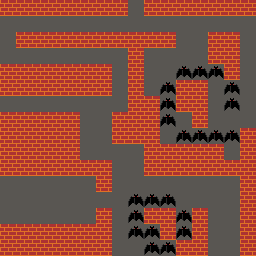}{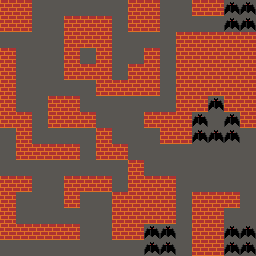} \\

\bottomrule
\end{tabular}
\vspace{-0.3cm}
\end{table*}

\begin{table*}[H]
\centering
\small

\caption{Examples from the AI dataset $\mathcal{D}_\mathrm{AI}$, illustrating various textual instructions and visualized levels for each task. Task conditions are highlighted in the text.}
\label{tab:dataset_ai}
\vspace{0.3cm}
\begin{tabular}{@{} p{3.3cm} p{8.5cm} p{4.2cm}@{}}
\toprule
\textbf{Task} & \textbf{Text}  & \textbf{Level} \\

\midrule 
\multirow{3}{*}{\raisebox{-4em}{\textbf{Number of Regions}}}
& \multirow{2}{*}{\shortstack[l]{
    \textbf{\textit{AI-generated layout}} featuring a \textbf{\textit{few\hidden{(5)}}} regions.\\
    \textbf{\textit{Sparse\hidden{(5)}}} regions, \textbf{\textit{arranged with artificial precision}}.%
  }
}
& \tripleimage{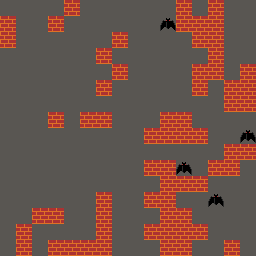}{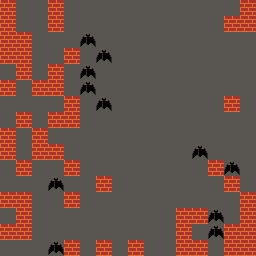}{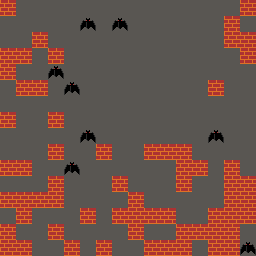} \vspace{0.03cm}\\

& \multirow{2}{*}{\shortstack[l]{
    An \textbf{\textit{AI-generated}} pattern of \textbf{\textit{some\hidden{(15)}}} clustered areas.\\
   \textbf{\textit{Moderately\hidden{(15)}}} dense layout of regions, \textbf{\textit{AI-style}}.%
  }
}
& \tripleimage{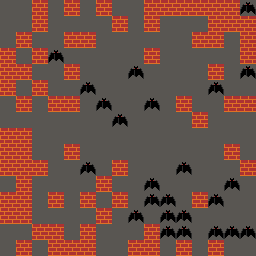}{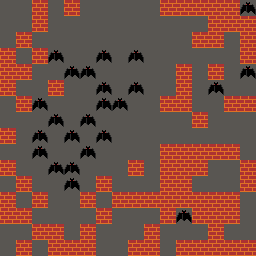}{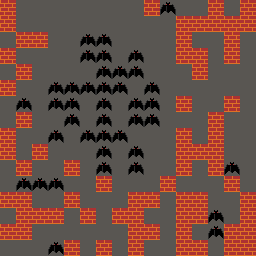} \vspace{0.03cm}\\

& \multirow{2}{*}{\shortstack[l]{
    \textbf{\textit{Several\hidden{(25)}}} regions with \textbf{\textit{AI-like arrangement}}.\\
   \textbf{\textit{Scattered\hidden{(25)}}} regions resembling \textbf{\textit{AI-generated structure}}.%
  }
}
& \tripleimage{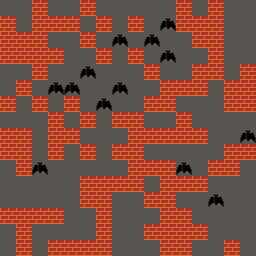}{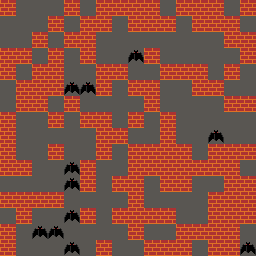}{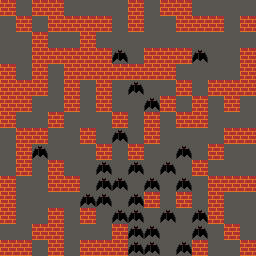} \\

\midrule 
\multirow{3}{*}{\raisebox{-4em}{\textbf{Path Length}}}
& \multirow{2}{*}{\shortstack[l]{
    \textbf{\textit{AI-generated}} route, \textbf{\textit{short and direct\hidden{(10)}}}.\\
    \textbf{\textit{Nano\hidden{(10)}}}-length path designed by \textbf{\textit{AI logic}}%
  }
}
&\tripleimage{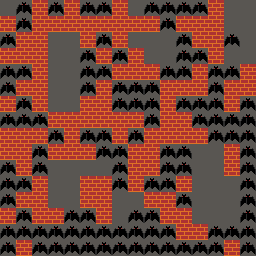}{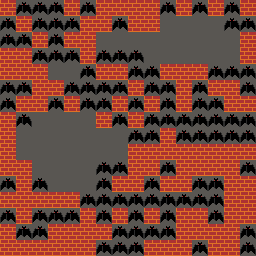}{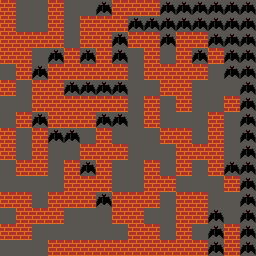} \vspace{0.03cm}\\

& \multirow{2}{*}{\shortstack[l]{
   \textbf{\textit{Compact\hidden{(20)}}} path layout in \textbf{\textit{AI style}}.\\
    \textbf{\textit{Short\hidden{(20)}}} path length with \textbf{\textit{AI design}}.%
  }
}
&\tripleimage{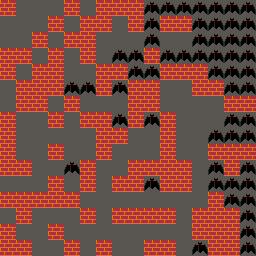}{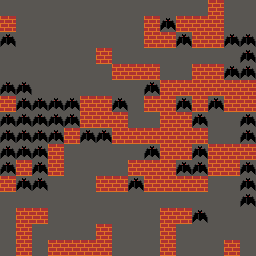}{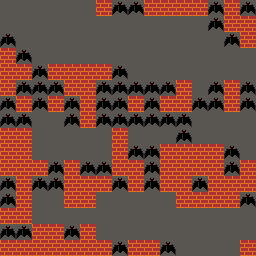} \vspace{0.03cm}\\

& \multirow{2}{*}{\shortstack[l]{
    \textbf{\textit{Moderate\hidden{(40)}}} path length with \textbf{\textit{AI-like design}}.\\
   \textbf{\textit{Medium\hidden{(40)}}}-length path in \textbf{\textit{AI-generated form}}.%
  }
}
&\tripleimage{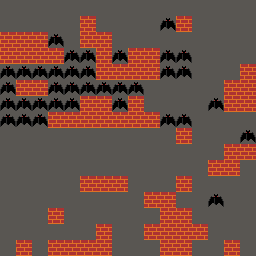}{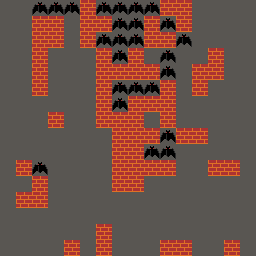}{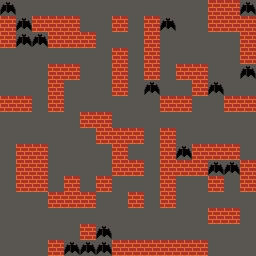} \\

\midrule 
\multirow{3}{*}{\raisebox{-4em}{\textbf{Wall Distribution}}}
& \multirow{2}{*}{\shortstack[l]{
    \textbf{\textit{Sparse\hidden{(40)}}} blocks in \textbf{\textit{AI-style layout}}.\\
    \textbf{\textit{Few\hidden{(40)}}} blocks in \textbf{\textit{AI-generated pattern}}.%
  }
}
&\tripleimage{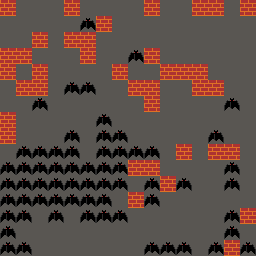}{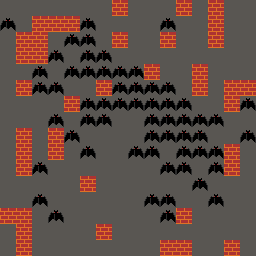}{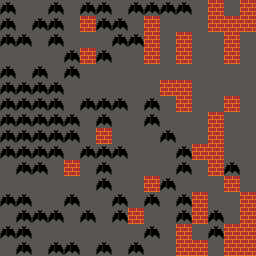} \vspace{0.03cm}\\

& \multirow{2}{*}{\shortstack[l]{
    \textbf{\textit{Some\hidden{(80)}}} blocks spread out in \textbf{\textit{AI layout}}.\\
   \textbf{\textit{Some\hidden{(80)}}} blocks follow \textbf{\textit{AI-style layout}}.%
  }
}
&\tripleimage{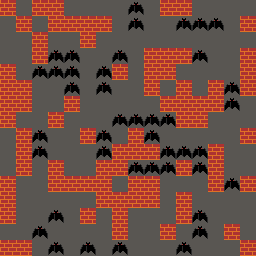}{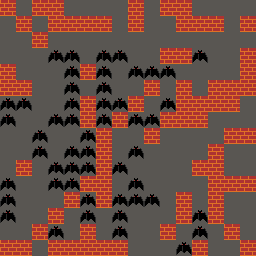}{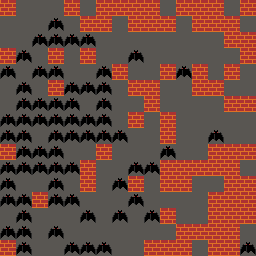} \vspace{0.03cm}\\

& \multirow{2}{*}{\shortstack[l]{
    \textbf{\textit{Numerous\hidden{(120)}}} blocks form \textbf{\textit{AI obstacle pattern}}.\\
   \textbf{\textit{Dense\hidden{(120)}}} blocks fill \textbf{\textit{AI-style layout}}.%
  }
}
&\tripleimage{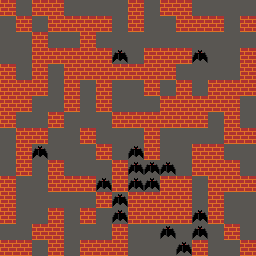}{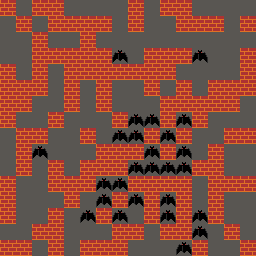}{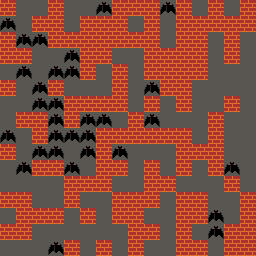}\\

\midrule 
\multirow{3}{*}{\raisebox{-4em}{\textbf{Monster Distribution}}}
& \multirow{2}{*}{\shortstack[l]{
    A \textbf{\textit{few\hidden{(10)}}} clustered bats form \textbf{\textit{AI-style layout}}.\\
    A \textbf{\textit{few\hidden{(10)}}} bats in \textbf{\textit{AI-like pattern}}.%
  }
}
&\tripleimage{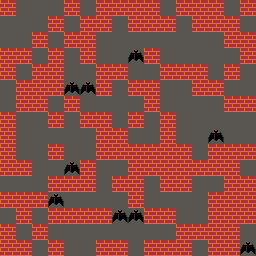}{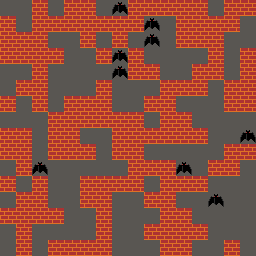}{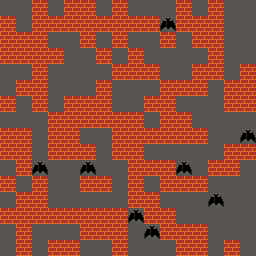} \vspace{0.03cm}\\

& \multirow{2}{*}{\shortstack[l]{
    \textbf{\textit{Some\hidden{(40)}}} bats spawn in \textbf{\textit{AI-like pattern}}.\\
   \textbf{\textit{Some\hidden{(40)}}} bats spread in \textbf{\textit{AI formation}}.%
  }
}
&\tripleimage{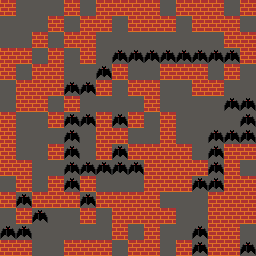}{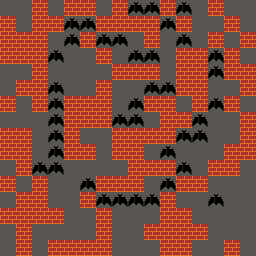}{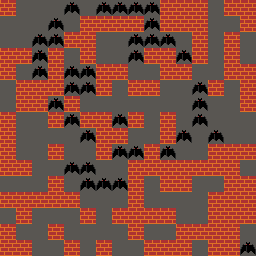} \vspace{0.03cm}\\

& \multirow{2}{*}{\shortstack[l]{
    \textbf{\textit{Several\hidden{(70)}}} bat swarm emerges with \textbf{\textit{AI-like design}}.\\
  \textbf{\textit{Several\hidden{(70)}}} bat groups dominates in \textbf{\textit{AI-style layout}}.%
  }
}
&\tripleimage{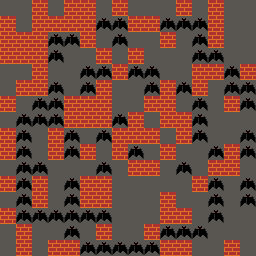}{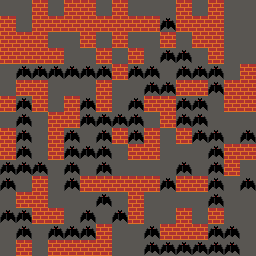}{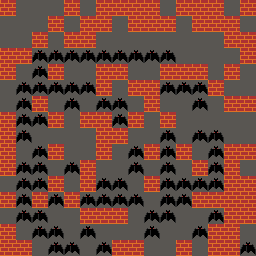}  \\

\midrule 
\multirow{3}{*}{\raisebox{-4em}{\textbf{Monster Direction}}}

& \multirow{2}{*}{\shortstack[l]{
   Bats cluster \textbf{\textit{west}} with \textbf{\textit{AI intent}}.\\
   \textbf{\textit{Left side}} bat spread, \textbf{\textit{AI-designed}}. %
  }
}
&\tripleimage{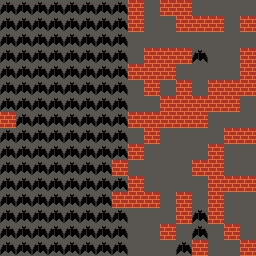}{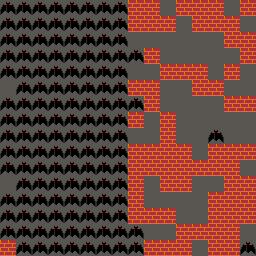}{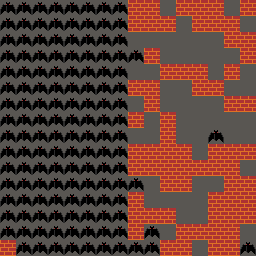} \vspace{0.03cm}\\

& \multirow{2}{*}{\shortstack[l]{
   \textbf{\textit{Top-focused}} bat group in \textbf{\textit{AI layout}}.\\
   Bats grouped \textbf{\textit{north}} with \textbf{\textit{AI intent}}.%
  }
}
&\tripleimage{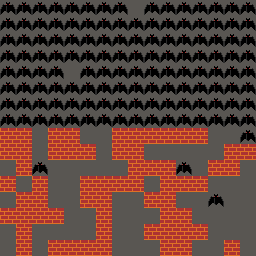}{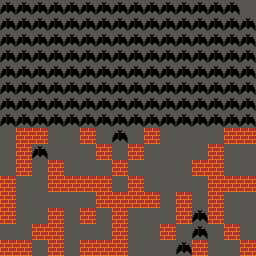}{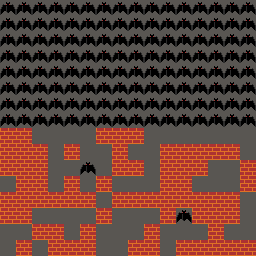} \vspace{0.03cm}\\

& \multirow{2}{*}{\shortstack[l]{
    Bat formation appears \textbf{\textit{right}}, \textbf{\textit{AI-guided}}.\\
   \textbf{\textit{Eastern}} bats follow \textbf{\textit{AI-like distribution}}.%
  }
}
&\tripleimage{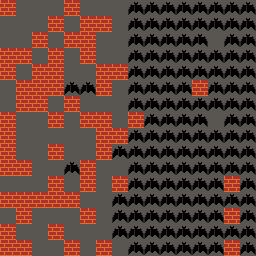}{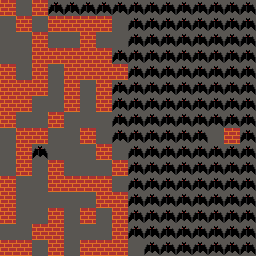}{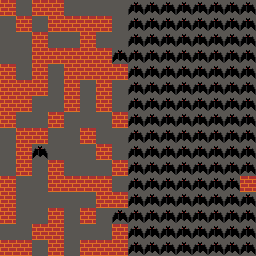} \\

\bottomrule
\end{tabular}
\vspace{-0.3cm}
\end{table*}
